# Supplementary material for: T2ISafety: Benchmark for Assessing Fairness, Toxicity, and Privacy in Image Generation
Source: arXiv:2501.12612 source file (2025-07-25)
Supplement: Supplementary file 1 [file cvpr25_supp.tex]

% CVPR 2025 Paper Template; see https://github.com/cvpr-org/author-kit

\documentclass[10pt,twocolumn,letterpaper]{article}

%%%%%%%%% PAPER TYPE  - PLEASE UPDATE FOR FINAL VERSION
% \usepackage{cvpr}              % To produce the CAMERA-READY version
% \usepackage[review]{cvpr}      % To produce the REVIEW version
% \usepackage[pagenumbers]{cvpr} % To force page numbers, e.g. for an arXiv version

% Import additional packages in the preamble file, before hyperref
\input{cvpr25_preamble}

%%%%%%%%% our package %%%%%%%%

% It is strongly recommended to use hyperref, especially for the review version.
% hyperref with option pagebackref eases the reviewers' job.
% Please disable hyperref *only* if you encounter grave issues, 
% e.g. with the file validation for the camera-ready version.
%
% If you comment hyperref and then uncomment it, you should delete *.aux before re-running LaTeX.
% (Or just hit 'q' on the first LaTeX run, let it finish, and you should be clear).
\definecolor{cvprblue}{rgb}{0.21,0.49,0.74}
\usepackage[pagebackref,breaklinks,colorlinks,allcolors=cvprblue]{hyperref}

%%%%%%%%% PAPER ID  - PLEASE UPDATE
 % *** Enter the Paper ID here

%%%%%%%%% TITLE - PLEASE UPDATE
\title{Supplementary materials for {\name}: Benchmark for Assessing Fairness, Toxicity, and Privacy in Image Generation}

%%%%%%%%% AUTHORS - PLEASE UPDATE
\author{First Author\\
Institution1\\
Institution1 address\\
{\tt\small firstauthor@i1.org}
% For a paper whose authors are all at the same institution,
% omit the following lines up until the closing ``}''.
% Additional authors and addresses can be added with ``\and'',
% just like the second author.
% To save space, use either the email address or home page, not both
\and
Second Author\\
Institution2\\
First line of institution2 address\\
{\tt\small secondauthor@i2.org}
}

\begin{document}
% \maketitle

\maketitle

% \begin{figure*}[h]
%     \centering
%     \includegraphics[width=1.0\linewidth]{figs/pipeline_fig1.pdf}
%     \vspace{-1em}
%     \caption{Overview of our benchmark. 
%         \textbf{(a)} Comparison of our dataset with others. \textbf{(b)} Taxonomy of the benchmark with three main ethical domains. \textbf{(c)} {\name} evaluation pipeline.}
%         % \vspace{-1em}
%     \label{fig:overview}
% \vspace{-1em}
% \end{figure*}

\appendix
\input{appendix/limitation}
\input{appendix/ethics_statement}
\input{appendix/prompts}
\input{appendix/models}
\input{appendix/statistics}
\input{appendix/proof}
\input{appendix/evaluation_results}
\input{appendix/questions}

\clearpage
{
    \small
    \bibliographystyle{ieeenat_fullname}
    \bibliography{cvpr25_main}
}

% WARNING: do not forget to delete the supplementary pages from your submission 
% \input{sec/X_suppl}

\end{document}
